# Supplementary material for: A multi-criteria approach for selecting an explanation from the set of counterfactuals produced by an ensemble of explainers
Source: arXiv:2403.13940 source file (2024-08-02)
Supplement: Supplementary file 1 [file appendix_generated_cfs.tex]

\definecolor{rest}{RGB}{52, 152, 219}
\definecolor{pareto}{RGB}{245, 176, 65}
\definecolor{nonactionable}{RGB}{149, 165, 166}
\definecolor{invalid}{RGB}{ 205, 97, 85 }
\definecolor{best}{RGB}{39, 174, 96}

\begin{table}[]
\tiny
    \centering
    \makebox[0cm]{

\begin{tabular}{rlrrrrrlllllll}
\hline
 ID & explainer &  age &  edu.num &  capital.gain &  capital.loss &  hrs/week &        workclass &     marital.status &        occupation &     race &  sex &    nat.cntry & income   \\  
\hline \hline
 \rowcolor{rest}
    1 &      dice & 24.0 &     10.0 &        5193.0 &           0.0 &      30.0 & Self-emp-not-inc &  Married-AF-spouse &    Prof-specialty & As-Pa-Is & Male &          USA &  <=50K   \\  \rowcolor{rest}
    2 &      dice & 24.0 &     10.0 &           0.0 &        3851.0 &      30.0 & Self-emp-not-inc &      Never-married &    Prof-specialty & As-Pa-Is & Male &          USA &  <=50K   \\  \rowcolor{pareto}
    3 &      dice & 24.0 &     10.0 &           0.0 &        3139.0 &      30.0 & Self-emp-not-inc &      Never-married &    Prof-specialty & As-Pa-Is & Male &          USA &  <=50K   \\  \rowcolor{rest}
    4 &      dice & 24.0 &      6.0 &       49751.0 &           0.0 &      30.0 & Self-emp-not-inc &      Never-married &    Prof-specialty & As-Pa-Is & Male &          USA &  <=50K   \\  \rowcolor{best}
    5 &      dice & 24.0 &     10.0 &       17327.0 &           0.0 &      30.0 & Self-emp-not-inc &      Never-married &    Prof-specialty & As-Pa-Is & Male &          USA &  <=50K   \\  \rowcolor{rest}
    6 &      dice & 24.0 &     10.0 &       26115.0 &        3511.0 &      30.0 & Self-emp-not-inc &      Never-married &    Prof-specialty & As-Pa-Is & Male &          USA &  <=50K   \\  \rowcolor{rest}
    7 &      dice & 24.0 &     10.0 &       94281.0 &           0.0 &      30.0 & Self-emp-not-inc &      Never-married &             Sales & As-Pa-Is & Male &          USA &  <=50K   \\  \rowcolor{pareto}
    8 &      dice & 24.0 &     10.0 &           0.0 &         402.0 &      30.0 & Self-emp-not-inc & Married-civ-spouse &    Prof-specialty & As-Pa-Is & Male &          USA &  <=50K   \\  \rowcolor{pareto}
    9 &      dice & 78.0 &     10.0 &           0.0 &           0.0 &      30.0 & Self-emp-not-inc &  Married-AF-spouse &    Prof-specialty & As-Pa-Is & Male &          USA &  <=50K   \\  \rowcolor{rest}
   10 &      dice & 24.0 &     10.0 &       29264.0 &           0.0 &      30.0 & Self-emp-not-inc &      Never-married &    Prof-specialty & As-Pa-Is & Male &          USA &  <=50K   \\  \rowcolor{rest}
   11 &      dice & 24.0 &     10.0 &           0.0 &           0.0 &      51.0 & Self-emp-not-inc &            Widowed &    Prof-specialty & As-Pa-Is & Male &          USA &  <=50K   \\  \rowcolor{pareto}
   12 &      dice & 24.0 &     10.0 &        4349.0 &           0.0 &      30.0 & Self-emp-not-inc &      Never-married &    Prof-specialty & As-Pa-Is & Male &          USA &  <=50K   \\  \rowcolor{rest}
   13 &      dice & 70.0 &     10.0 &       53380.0 &           0.0 &      30.0 & Self-emp-not-inc &      Never-married &    Prof-specialty & As-Pa-Is & Male &          USA &  <=50K   \\  \rowcolor{pareto}
   14 &      dice & 54.0 &     10.0 &           0.0 &           0.0 &      30.0 & Self-emp-not-inc & Married-civ-spouse &    Prof-specialty & As-Pa-Is & Male &          USA &  <=50K   \\  \rowcolor{rest}
   15 &      dice & 24.0 &     14.0 &       10377.0 &           0.0 &      30.0 & Self-emp-not-inc &      Never-married &    Prof-specialty & As-Pa-Is & Male &          USA &  <=50K   \\  \rowcolor{rest}
   16 &      dice & 39.0 &     10.0 &           0.0 &        3097.0 &      30.0 & Self-emp-not-inc &      Never-married &    Prof-specialty & As-Pa-Is & Male &          USA &  <=50K   \\  \rowcolor{rest}
   17 &      dice & 24.0 &     10.0 &       66733.0 &           0.0 &      30.0 & Self-emp-not-inc &      Never-married &    Prof-specialty & As-Pa-Is & Male &          USA &  <=50K   \\  \rowcolor{rest}
   18 &      dice & 24.0 &     10.0 &           0.0 &        4354.0 &      30.0 & Self-emp-not-inc &      Never-married &    Prof-specialty & As-Pa-Is & Male &          USA &  <=50K   \\  \rowcolor{rest}
   19 &      dice & 24.0 &     10.0 &           0.0 &        3568.0 &      30.0 & Self-emp-not-inc &      Never-married &    Prof-specialty & As-Pa-Is & Male &          USA &  <=50K   \\  \rowcolor{rest}
   20 &      dice & 24.0 &     10.0 &           0.0 &        4207.0 &      30.0 & Self-emp-not-inc &      Never-married &    Prof-specialty & As-Pa-Is & Male &          USA &  <=50K   \\  \rowcolor{rest}
   21 &     cadex & 24.0 &     10.0 &        4999.0 &           0.0 &      30.0 & Self-emp-not-inc &      Never-married &    Prof-specialty & As-Pa-Is & Male &          USA &  <=50K   \\  \rowcolor{pareto}
   22 &     cadex & 27.0 &     10.0 &        4999.0 &           0.0 &      30.0 & Self-emp-not-inc &      Never-married &    Prof-specialty & As-Pa-Is & Male &          USA &  <=50K   \\  \rowcolor{pareto}
   23 &     cadex & 27.0 &     10.0 &        4999.0 &           0.0 &      34.0 & Self-emp-not-inc &      Never-married &    Prof-specialty & As-Pa-Is & Male &          USA &  <=50K   \\  \rowcolor{rest}
   24 &     cadex & 27.0 &     10.0 &        4999.0 &         217.0 &      34.0 & Self-emp-not-inc &      Never-married &    Prof-specialty & As-Pa-Is & Male &          USA &  <=50K   \\  \rowcolor{rest}
   25 &     cadex & 27.0 &     10.0 &        4999.0 &         217.0 &      34.0 & Self-emp-not-inc &      Never-married &    Prof-specialty & As-Pa-Is & Male &          USA &  <=50K   \\  \rowcolor{pareto}
   26 &     fimap & 30.0 &     11.0 &       10317.0 &         102.0 &      34.0 &          Private & Married-civ-spouse &    Prof-specialty & As-Pa-Is & Male &          USA &  <=50K   \\  \rowcolor{pareto}
   27 &     fimap & 30.0 &     10.0 &        5907.0 &          43.0 &      32.0 &          Private & Married-civ-spouse &    Prof-specialty & As-Pa-Is & Male &          USA &  <=50K   \\  \rowcolor{pareto}
   28 &     fimap & 31.0 &     10.0 &        6444.0 &          49.0 &      32.0 &          Private & Married-civ-spouse & Machine-op-inspct & As-Pa-Is & Male &          USA &  <=50K   \\  \rowcolor{rest}
   29 &     fimap & 31.0 &     11.0 &        9949.0 &         102.0 &      33.0 &          Private & Married-civ-spouse & Handlers-cleaners & As-Pa-Is & Male &          USA &  <=50K   \\  \rowcolor{rest}
   30 &     fimap & 31.0 &     11.0 &        7127.0 &          61.0 &      32.0 &          Private &           Divorced &    Prof-specialty & As-Pa-Is & Male &          USA &  <=50K   \\  \rowcolor{invalid}
   31 &     fimap & 31.0 &     10.0 &        6595.0 &          49.0 &      32.0 &          Private &           Divorced &                 ? & As-Pa-Is & Male &          USA &   >50K   \\  \rowcolor{rest}
   32 &   wachter & 72.0 &     10.0 &        3885.0 &           0.0 &      65.0 & Self-emp-not-inc &      Never-married &    Prof-specialty & As-Pa-Is & Male &          USA &  <=50K   \\  \rowcolor{rest}
   33 &   wachter & 70.0 &      9.0 &        3640.0 &           0.0 &      55.0 & Self-emp-not-inc &      Never-married &    Prof-specialty & As-Pa-Is & Male &          USA &  <=50K   \\  \rowcolor{invalid}
   34 &   wachter & 53.0 &      9.0 &        2918.0 &           0.0 &      33.0 & Self-emp-not-inc &      Never-married &    Prof-specialty & As-Pa-Is & Male &          USA &   >50K   \\  \rowcolor{rest}
   35 &   wachter & 24.0 &     10.0 &        4402.0 &           0.0 &      29.0 & Self-emp-not-inc &      Never-married &    Prof-specialty & As-Pa-Is & Male &          USA &  <=50K   \\  \rowcolor{invalid}
   36 &   wachter & 31.0 &      9.0 &        2614.0 &           1.0 &      30.0 & Self-emp-not-inc &      Never-married &    Prof-specialty & As-Pa-Is & Male &          USA &   >50K   \\  \rowcolor{rest}
   37 &   wachter & 24.0 &     10.0 &        4469.0 &           0.0 &      30.0 & Self-emp-not-inc &      Never-married &    Prof-specialty & As-Pa-Is & Male &          USA &  <=50K   \\  \rowcolor{invalid}
   38 &   wachter & 23.0 &      9.0 &        4474.0 &           0.0 &      29.0 & Self-emp-not-inc &      Never-married &    Prof-specialty & As-Pa-Is & Male &          USA &   >50K   \\  \rowcolor{pareto}
   39 &   wachter & 70.0 &     10.0 &        3712.0 &           0.0 &      62.0 & Self-emp-not-inc &      Never-married &    Prof-specialty & As-Pa-Is & Male &          USA &  <=50K   \\  \rowcolor{rest}
   40 &   wachter & 58.0 &      8.0 &        4964.0 &           0.0 &      34.0 & Self-emp-not-inc &      Never-married &    Prof-specialty & As-Pa-Is & Male &          USA &  <=50K   \\  \rowcolor{invalid}
   41 &   wachter & 23.0 &     10.0 &        4405.0 &           0.0 &      30.0 & Self-emp-not-inc &      Never-married &    Prof-specialty & As-Pa-Is & Male &          USA &   >50K   \\  \rowcolor{rest}
   42 &       cem & 24.0 &     10.0 &        5939.0 &           0.0 &      30.0 & Self-emp-not-inc &      Never-married &    Prof-specialty & As-Pa-Is & Male &          USA &  <=50K   \\  \rowcolor{nonactionable}
   43 &   cfproto & 24.0 &     10.0 &       15154.0 &           0.0 &      30.0 &     Self-emp-inc &      Never-married &   Protective-serv & As-Pa-Is & Male &       France &  <=50K   \\  \rowcolor{nonactionable}
   44 &   cfproto & 28.0 &     10.0 &       35794.0 &           0.0 &      30.0 &                ? &      Never-married &   Protective-serv &    White & Male & Outlying-US( &  <=50K   \\  \rowcolor{nonactionable}
   45 &   cfproto & 24.0 &     10.0 &       13763.0 &           0.0 &      30.0 & Self-emp-not-inc &      Never-married &    Prof-specialty &    White & Male &  Philippines &  <=50K   \\  \rowcolor{nonactionable}
   46 &   cfproto & 24.0 &     10.0 &       18256.0 &           0.0 &      30.0 &     Self-emp-inc &      Never-married &    Prof-specialty &    White & Male &        China &  <=50K   \\  \rowcolor{nonactionable}
   47 &   cfproto & 24.0 &     10.0 &       34508.0 &           0.0 &      30.0 &     Self-emp-inc &      Never-married &    Prof-specialty &    White & Male &      Vietnam &  <=50K   \\  \rowcolor{nonactionable}
   48 &   cfproto & 24.0 &     10.0 &       40939.0 &           0.0 &      30.0 &        State-gov &      Never-married &    Prof-specialty &    White & Male &        India &  <=50K   \\  \rowcolor{nonactionable}
   49 &   cfproto & 24.0 &     10.0 &       26873.0 &           0.0 &      30.0 &     Self-emp-inc &      Never-married &    Prof-specialty &    White & Male &        China &  <=50K   \\  \rowcolor{nonactionable}
   50 &   cfproto & 23.0 &     10.0 &       45951.0 &           0.0 &      30.0 &      Without-pay &      Never-married &    Prof-specialty &    White & Male &       Greece &  <=50K   \\  \rowcolor{nonactionable}
   51 &   cfproto & 24.0 &     10.0 &       13763.0 &           0.0 &      30.0 & Self-emp-not-inc &      Never-married &    Prof-specialty &    White & Male &  Philippines &  <=50K   \\  \rowcolor{rest}
   52 &  grow-sph & 45.0 &      9.0 &       26255.0 &         703.0 &      22.0 &      Federal-gov & Married-civ-spouse &                 ? & As-Pa-Is & Male &          USA &  <=50K   \\  \rowcolor{rest}
   53 &  grow-sph & 17.0 &     14.0 &       42417.0 &          86.0 &      36.0 &     Self-emp-inc &           Divorced &                 ? & As-Pa-Is & Male &          USA &  <=50K   \\  \rowcolor{rest}
   54 &  grow-sph & 34.0 &     10.0 &       26651.0 &         333.0 &      27.0 &                ? &           Divorced &                 ? & As-Pa-Is & Male &          USA &  <=50K   \\  \rowcolor{rest}
   55 &  grow-sph & 30.0 &     13.0 &       31719.0 &        1324.0 &      24.0 &                ? &           Divorced &                 ? & As-Pa-Is & Male &          USA &  <=50K   \\  \rowcolor{rest}
   56 &  grow-sph & 17.0 &      9.0 &       29154.0 &          47.0 &      43.0 &          Private &  Married-AF-spouse &      Armed-Forces & As-Pa-Is & Male &          USA &  <=50K   \\  \rowcolor{rest}
   57 &  grow-sph & 46.0 &     12.0 &       17359.0 &           0.0 &      36.0 &                ? &  Married-AF-spouse &      Craft-repair & As-Pa-Is & Male &          USA &  <=50K   \\  \rowcolor{rest}
   58 &  grow-sph & 17.0 &      9.0 &       19830.0 &           0.0 &      36.0 &      Federal-gov &  Married-AF-spouse &      Adm-clerical & As-Pa-Is & Male &          USA &  <=50K   \\  \rowcolor{rest}
   59 &  grow-sph & 24.0 &      6.0 &       22589.0 &         115.0 &      24.0 &                ? &  Married-AF-spouse &      Craft-repair & As-Pa-Is & Male &          USA &  <=50K   \\  \rowcolor{rest}
   60 &  grow-sph & 33.0 &      8.0 &       25089.0 &         552.0 &      29.0 &      Federal-gov &           Divorced &      Armed-Forces & As-Pa-Is & Male &          USA &  <=50K   \\  \rowcolor{rest}
   61 &  grow-sph & 29.0 &     10.0 &       31798.0 &         215.0 &      30.0 &      Federal-gov &           Divorced &      Adm-clerical & As-Pa-Is & Male &          USA &  <=50K   \\  \rowcolor{rest}
   62 &  grow-sph & 17.0 &      8.0 &       49887.0 &         641.0 &      52.0 &                ? &  Married-AF-spouse &      Craft-repair & As-Pa-Is & Male &          USA &  <=50K   \\  \rowcolor{rest}
   63 &  grow-sph & 30.0 &     10.0 &       35880.0 &           0.0 &      33.0 &      Federal-gov &           Divorced &      Craft-repair & As-Pa-Is & Male &          USA &  <=50K   \\  \rowcolor{rest}
   64 &  grow-sph & 21.0 &     10.0 &       27720.0 &           0.0 &      35.0 &                ? &           Divorced &                 ? & As-Pa-Is & Male &          USA &  <=50K   \\  \rowcolor{rest}
   65 &  grow-sph & 31.0 &      7.0 &       47001.0 &         198.0 &      22.0 &          Private &  Married-AF-spouse &      Adm-clerical & As-Pa-Is & Male &          USA &  <=50K   \\  \rowcolor{rest}
   66 &  grow-sph & 25.0 &     11.0 &       24283.0 &         518.0 &      15.0 &                ? &           Divorced &      Craft-repair & As-Pa-Is & Male &          USA &  <=50K   \\  \rowcolor{rest}
   67 &  grow-sph & 40.0 &      7.0 &       36015.0 &         275.0 &       5.0 &      Federal-gov &           Divorced &      Armed-Forces & As-Pa-Is & Male &          USA &  <=50K   \\  \rowcolor{rest}
   68 &  grow-sph & 32.0 &      9.0 &       29964.0 &           0.0 &      36.0 & Self-emp-not-inc &           Divorced & Machine-op-inspct & As-Pa-Is & Male &          USA &  <=50K   \\  \rowcolor{rest}
   69 &  grow-sph & 39.0 &     11.0 &       20938.0 &           0.0 &      38.0 &      Federal-gov &  Married-AF-spouse &   Farming-fishing & As-Pa-Is & Male &          USA &  <=50K   \\  \rowcolor{rest}
   70 &  grow-sph & 35.0 &     10.0 &       34992.0 &           0.0 &      67.0 &          Private &  Married-AF-spouse & Machine-op-inspct & As-Pa-Is & Male &          USA &  <=50K   \\  \rowcolor{rest}
   71 &  grow-sph & 17.0 &      3.0 &       30575.0 &         430.0 &      26.0 &          Private &  Married-AF-spouse &   Exec-managerial & As-Pa-Is & Male &          USA &  <=50K   \\  \rowcolor{rest}
   72 &   act-rec & 24.0 &     10.0 &           0.0 &           0.0 &      29.0 & Self-emp-not-inc &  Married-AF-spouse &    Prof-specialty & As-Pa-Is & Male &          USA &  <=50K   \\  \rowcolor{nonactionable}
   73 &      face & 32.0 &     14.0 &           0.0 &           0.0 &      39.0 & Self-emp-not-inc &      Never-married &    Prof-specialty &    White & Male &          USA &  <=50K   \\  \rowcolor{nonactionable}
   74 &      face & 39.0 &     16.0 &        4787.0 &           0.0 &      39.0 & Self-emp-not-inc &      Never-married &    Prof-specialty &    White & Male &          USA &  <=50K   \\  \rowcolor{pareto}
   75 &      face & 27.0 &     13.0 &       13549.0 &           0.0 &      39.0 &          Private &      Never-married &    Prof-specialty & As-Pa-Is & Male &          USA &  <=50K   \\  \rowcolor{nonactionable}
   76 &      face & 37.0 &     13.0 &           0.0 &           0.0 &      39.0 & Self-emp-not-inc & Married-civ-spouse &    Prof-specialty &    White & Male &          USA &  <=50K   \\  \rowcolor{nonactionable}
   77 &      face & 38.0 &     10.0 &        3137.0 &           0.0 &      50.0 & Self-emp-not-inc & Married-civ-spouse &    Prof-specialty &    White & Male &          USA &  <=50K   \\  \rowcolor{nonactionable}
   78 &      face & 35.0 &      9.0 &        8614.0 &           0.0 &      39.0 & Self-emp-not-inc &      Never-married & Machine-op-inspct &    White & Male &          USA &  <=50K   \\  \rowcolor{nonactionable}
   79 &      face & 30.0 &     15.0 &           0.0 &           0.0 &      39.0 & Self-emp-not-inc &      Never-married &    Prof-specialty &    White & Male &          USA &  <=50K   \\  \rowcolor{nonactionable}
   80 &      face & 35.0 &     13.0 &           0.0 &           0.0 &      39.0 & Self-emp-not-inc & Married-civ-spouse &    Prof-specialty &    White & Male &          USA &  <=50K   \\  \rowcolor{nonactionable}
   81 &      face & 39.0 &     14.0 &           0.0 &           0.0 &      39.0 & Self-emp-not-inc &      Never-married &    Prof-specialty &    White & Male &          USA &  <=50K   \\  \rowcolor{nonactionable}
   82 &      face & 37.0 &      9.0 &        3137.0 &           0.0 &      29.0 & Self-emp-not-inc & Married-civ-spouse &    Prof-specialty &    White & Male &          USA &  <=50K   \\  
\hline
\end{tabular}

}
       \caption{Full list of generated counterfactual explanations for the toy example.}
   \label{tab:appendix-all-toy-cfs}
\end{table}
