# Supplementary material for: A multi-criteria approach for selecting an explanation from the set of counterfactuals produced by an ensemble of explainers
Source: arXiv:2403.13940 source file (2024-08-02)
Supplement: Supplementary file 2 [file appendix_scores.tex]

\begin{table}[]
\tiny
    \centering
    \makebox[0cm]{
    \begin{tabular}{l|l|l|l|l}
    \hline
       ID & Proximity & K\_Feasibility(3) & DiscriminativePower(9) & explainer \\ \hline
        1 & 1.052 & 1.506 & 0.222 & dice \\ \hline
        2 & 0.884 & 1.491 & 0.222 & dice \\ \hline
        3 & 0.721 & 1.328 & 0.222 & dice \\ \hline
        4 & 0.764 & 1.517 & 0.000 & dice \\ \hline
        5 & 0.173 & 0.962 & 0.111 & dice \\ \hline
        6 & 1.067 & 1.674 & 0.222 & dice \\ \hline
        7 & 1.943 & 1.529 & 0.111 & dice \\ \hline
        8 & 1.092 & 1.093 & 0.444 & dice \\ \hline
        9 & 1.740 & 1.975 & 0.667 & dice \\ \hline
        10 & 0.293 & 1.082 & 0.111 & dice \\ \hline
        11 & 1.214 & 1.475 & 0.444 & dice \\ \hline
        12 & 0.043 & 0.832 & 0.000 & dice \\ \hline
        13 & 1.164 & 1.706 & 0.111 & dice \\ \hline
        14 & 1.411 & 1.004 & 0.556 & dice \\ \hline
        15 & 0.370 & 0.966 & 0.111 & dice \\ \hline
        16 & 0.916 & 1.372 & 0.222 & dice \\ \hline
        17 & 0.667 & 1.456 & 0.111 & dice \\ \hline
        18 & 1.000 & 1.607 & 0.222 & dice \\ \hline
        19 & 0.819 & 1.426 & 0.222 & dice \\ \hline
        20 & 0.966 & 1.573 & 0.222 & dice \\ \hline
        21 & 0.050 & 0.839 & 0.000 & cadex \\ \hline
        22 & 0.091 & 0.825 & 0.000 & cadex \\ \hline
        23 & 0.132 & 0.812 & 0.000 & cadex \\ \hline
        24 & 0.182 & 0.861 & 0.000 & cadex \\ \hline
        25 & 0.182 & 0.861 & 0.000 & cadex \\ \hline
        26 & 2.316 & 0.608 & 1.000 & fimap \\ \hline
        27 & 2.172 & 0.633 & 0.889 & fimap \\ \hline
        28 & 3.192 & 0.595 & 0.667 & fimap \\ \hline
        29 & 3.316 & 0.879 & 0.333 & fimap \\ \hline
        30 & 2.268 & 1.212 & 0.000 & fimap \\ \hline
        31 & 3.193 & 1.522 & 0.667 & fimap \\ \hline
        32 & 1.054 & 1.331 & 0.222 & wachter \\ \hline
        33 & 0.988 & 1.255 & 0.111 & wachter \\ \hline
        34 & 0.524 & 1.002 & 1.000 & wachter \\ \hline
        35 & 0.054 & 0.843 & 0.000 & wachter \\ \hline
        36 & 0.189 & 0.883 & 1.000 & wachter \\ \hline
        37 & 0.045 & 0.834 & 0.000 & wachter \\ \hline
        38 & 0.135 & 0.882 & 1.000 & wachter \\ \hline
        39 & 0.994 & 1.271 & 0.222 & wachter \\ \hline
        40 & 0.690 & 1.148 & 0.000 & wachter \\ \hline
        41 & 0.058 & 0.846 & 1.000 & wachter \\ \hline
        42 & 0.059 & 0.848 & 0.000 & cem \\ \hline
        43 & 3.152 & 2.348 & 0.000 & cfproto \\ \hline
        44 & 4.413 & 2.433 & 0.000 & cfproto \\ \hline
        45 & 2.138 & 1.287 & 0.000 & cfproto \\ \hline
        46 & 3.183 & 1.537 & 0.333 & cfproto \\ \hline
        47 & 3.345 & 1.700 & 0.333 & cfproto \\ \hline
        48 & 3.409 & 1.528 & 0.000 & cfproto \\ \hline
        49 & 3.269 & 1.624 & 0.333 & cfproto \\ \hline
        50 & 3.473 & 2.513 & 0.111 & cfproto \\ \hline
        51 & 2.138 & 1.287 & 0.000 & cfproto \\ \hline
        52 & 3.860 & 1.812 & 0.778 & growing-spheres \\ \hline
        53 & 3.868 & 2.419 & 0.333 & growing-spheres \\ \hline
        54 & 3.511 & 1.218 & 0.000 & growing-spheres \\ \hline
        55 & 3.965 & 1.671 & 0.000 & growing-spheres \\ \hline
        56 & 3.598 & 2.397 & 0.222 & growing-spheres \\ \hline
        57 & 3.670 & 2.317 & 0.778 & growing-spheres \\ \hline
        58 & 3.422 & 1.778 & 0.111 & growing-spheres \\ \hline
        59 & 3.580 & 2.658 & 0.556 & growing-spheres \\ \hline
        60 & 3.644 & 2.278 & 0.111 & growing-spheres \\ \hline
        61 & 3.436 & 1.545 & 0.000 & growing-spheres \\ \hline
        62 & 4.100 & 2.984 & 0.778 & growing-spheres \\ \hline
        63 & 3.472 & 1.571 & 0.222 & growing-spheres \\ \hline
        64 & 3.369 & 1.270 & 0.000 & growing-spheres \\ \hline
        65 & 3.893 & 1.846 & 0.222 & growing-spheres \\ \hline
        66 & 3.595 & 2.119 & 0.333 & growing-spheres \\ \hline
        67 & 4.098 & 2.573 & 0.111 & growing-spheres \\ \hline
        68 & 2.537 & 1.689 & 0.222 & growing-spheres \\ \hline
        69 & 3.563 & 2.320 & 0.556 & growing-spheres \\ \hline
        70 & 3.878 & 1.665 & 0.556 & growing-spheres \\ \hline
        71 & 4.008 & 2.249 & 0.444 & growing-spheres \\ \hline
        72 & 1.010 & 1.519 & 0.222 & actionable-recourse \\ \hline
        73 & 1.468 & 0.056 & 0.667 & face \\ \hline
        74 & 1.745 & 0.128 & 1.000 & face \\ \hline
        75 & 1.468 & 0.110 & 0.111 & face \\ \hline
        76 & 2.470 & 0.028 & 1.000 & face \\ \hline
        77 & 2.427 & 0.084 & 1.000 & face \\ \hline
        78 & 2.395 & 0.191 & 0.111 & face \\ \hline
        79 & 1.507 & 0.058 & 0.778 & face \\ \hline
        80 & 2.443 & 0.019 & 1.000 & face \\ \hline
        81 & 1.564 & 0.047 & 0.667 & face \\ \hline
        82 & 2.286 & 0.121 & 0.667 & face \\ \hline
    \end{tabular}
    }
   \caption{The values of selected quality measures computed for counterfactual explanations in the toy example. IDs correspond to counterfactuals presented in Tab.~\ref{tab:appendix-all-toy-cfs}}
   \label{tab:appendix-all-toy-scores}
\end{table}
