# Supplementary material for: A multi-criteria approach for selecting an explanation from the set of counterfactuals produced by an ensemble of explainers
Source: arXiv:2403.13940 source file (2024-08-02)
Supplement: Supplementary file 3 [file elements_study_no_dominance_nadir.tex]

\begin{table}[!ht]
    \centering
    \caption{\textbf{Dataset}: German. \textbf{Setting}: Ensemble - Filtering - Dominance Relation - Nadir Selection. \textbf{Removed element}: None }
    \makebox[0cm]{
    
   \begin{tabular}{|l|l|l|l|l|l|l|l|l|}
    \hline
        \textbf{Method} & \textbf{proximity} & \textbf{feasibility} & \textbf{discriminative\_power} & \textbf{sparsity} & \textbf{instability} & \textbf{coverage} & \textbf{actionable} & \textbf{rank} \\ \hline
        \textbf{dice} & 1.92 & 4.11 & 0.46 & 2.18 & 4.3 & 1 & 1 & 3.14 \\ \hline
        \textbf{cadex} & 1.35 & 3.76 & 0.41 & 2.61 & 3.93 & 0.97 & 0.97 & 5.71 \\ \hline
        \textbf{fimap} & 6.75 & 3.07 & 0.55 & 9.79 & 3.79 & 0.97 & 0.97 & 5 \\ \hline
        \textbf{wachter} & 1.27 & 3.73 & 0.34 & 3.97 & 3.98 & 0.3 & 0.3 & 6.71 \\ \hline
        \textbf{cem} & 0.62 & 4.18 & 0.31 & 2.15 & 3.99 & 0.13 & 0.13 & 7.43 \\ \hline
        \textbf{cfproto} & 4.05 & 4.54 & 0.49 & 5.43 & 4.74 & 0.93 & 0.93 & 5.86 \\ \hline
        \textbf{growing-spheres} & 7.51 & 5.82 & 0.59 & 10.56 & 5.6 & 1 & 1 & 2.57 \\ \hline
        \textbf{actionable-recourse} & 1.01 & 3.55 & 0.44 & 1.39 & 3.6 & 0.23 & 0.23 & 6.71 \\ \hline
        \textbf{face} & 5.11 & 1.89 & 0.62 & 8.16 & 3.79 & 0.99 & 0.99 & 4.43 \\ \hline
        \textbf{ip-manhattan} & 3.83 & 2.15 & 0.85 & 6.06 & 3.5 & 1 & 1 & 1.86 \\ \hline
        \textbf{ip-euclidean} & 3.34 & 2.38 & 0.82 & 5.27 & 3.57 & 1 & 1 & 2.14 \\ \hline
        \textbf{ip-chebyshev} & 2.87 & 2.65 & 0.76 & 4.43 & 3.74 & 1 & 1 & 2.29 \\ \hline
        \textbf{s-bd} & 3.83 & 2.15 & 0.85 & 6.06 & 3.5 & 1 & 1 & 1.86 \\ \hline
        \textbf{rc-bd} & 4.51 & 4.21 & 0.5 & 6.38 & 4.57 & 1 & 1 & 2.86 \\ \hline
    \end{tabular}
    
    }
\end{table}

\begin{table}[!ht]
    \centering
    \caption{\textbf{Dataset}: Adult. \textbf{Setting}: Ensemble - Filtering - Dominance Relation - Nadir Selection. \textbf{Removed element}: None }
    \makebox[0cm]{
    
    \begin{tabular}{|l|l|l|l|l|l|l|l|l|}
    \hline
        \textbf{Method} & \textbf{proximity} & \textbf{feasibility} & \textbf{discriminative\_power} & \textbf{sparsity} & \textbf{instability} & \textbf{coverage} & \textbf{actionable} & \textbf{rank} \\ \hline
        \textbf{dice} & 1.14 & 0.86 & 0.34 & 1.7 & 1.2 & 1 & 1 & 3.29 \\ \hline
        \textbf{fimap} & 2.06 & 0.38 & 0.57 & 5.72 & 1.15 & 0.99 & 0.99 & 4.29 \\ \hline
        \textbf{cadex} & 0.2 & 0.3 & 0.17 & 2.29 & 0.64 & 0.99 & 0.99 & 5.29 \\ \hline
        \textbf{wachter} & 0.72 & 0.41 & 0.32 & 3.16 & 0.81 & 0.81 & 0.81 & 6.29 \\ \hline
        \textbf{cem} & 0.13 & 0.32 & 0.17 & 1.16 & 0.67 & 0.66 & 0.66 & 6.71 \\ \hline
        \textbf{cfproto} & 1.12 & 0.66 & 0.36 & 2.09 & 1.17 & 0.39 & 0.39 & 6.43 \\ \hline
        \textbf{growing-spheres} & 2.76 & 1.34 & 0.45 & 6.08 & 1.63 & 0.99 & 0.99 & 4.43 \\ \hline
        \textbf{face} & 1.02 & 0.11 & 0.68 & 3.67 & 0.63 & 0.93 & 0.93 & 5 \\ \hline
        \textbf{actionable-recourse} & 0.98 & 0.9 & 0.36 & 1.92 & 1.1 & 0.1 & 0.1 & 6.71 \\ \hline
        \textbf{ip-manhattan} & 1.02 & 0.17 & 0.94 & 3.34 & 0.63 & 1 & 1 & 1.86 \\ \hline
        \textbf{ip-euclidean} & 0.99 & 0.19 & 0.94 & 3.23 & 0.63 & 1 & 1 & 1.86 \\ \hline
        \textbf{ip-chebyshev} & 0.98 & 0.24 & 0.91 & 3.14 & 0.65 & 1 & 1 & 2.29 \\ \hline
        \textbf{s-bd} & 1.02 & 0.17 & 0.94 & 3.34 & 0.63 & 1 & 1 & 1.86 \\ \hline
        \textbf{rc-bd} & 1.54 & 0.78 & 0.41 & 3.74 & 1.15 & 1 & 1 & 2.86 \\ \hline
    \end{tabular}
    
    }
\end{table}

\begin{table}[!ht]
    \centering
    \caption{\textbf{Dataset}: Fico.  \textbf{Setting}: Ensemble - Filtering - Dominance Relation - Nadir Selection. \textbf{Removed element}: None }
    \makebox[0cm]{
    
    \begin{tabular}{|l|l|l|l|l|l|l|l|l|}
    \hline
        \textbf{Method} & \textbf{proximity} & \textbf{feasibility} & \textbf{discriminative\_power} & \textbf{sparsity} & \textbf{instability} & \textbf{coverage} & \textbf{actionable} & \textbf{rank} \\ \hline
        \textbf{dice} & 1.15 & 2.17 & 0.36 & 2.1 & 2.54 & 1 & 1 & 3.29 \\ \hline
        \textbf{cadex} & 0.94 & 1.71 & 0.38 & 7.82 & 2.03 & 1 & 1 & 3.14 \\ \hline
        \textbf{fimap} & 1.63 & 1.82 & 0.62 & 15.97 & 1.91 & 0.62 & 0.62 & 5.14 \\ \hline
        \textbf{wachter} & 0.91 & 1.66 & 0.33 & 13.66 & 1.88 & 0.99 & 0.99 & 5.86 \\ \hline
        \textbf{cem} & 1.12 & 2.08 & 0.5 & 5.8 & 2.47 & 1 & 1 & 2.71 \\ \hline
        \textbf{cfproto} & 0.66 & 1.54 & 0.42 & 9.32 & 1.77 & 0.58 & 0.58 & 6 \\ \hline
        \textbf{growing-spheres} & 1.43 & 1.91 & 0.34 & 16.33 & 2.41 & 0.97 & 0.97 & 6 \\ \hline
        \textbf{face} & 2.08 & 0.84 & 0.66 & 16.54 & 1.82 & 0.24 & 0.24 & 5.29 \\ \hline
        \textbf{ip-manhattan} & 0.87 & 1.51 & 0.6 & 7.33 & 1.89 & 1 & 1 & 2.43 \\ \hline
        \textbf{ip-euclidean} & 0.88 & 1.57 & 0.63 & 7.28 & 1.92 & 1 & 1 & 2 \\ \hline
        \textbf{ip-chebyshev} & 0.94 & 1.6 & 0.63 & 7.28 & 1.93 & 1 & 1 & 2 \\ \hline
        \textbf{s-bd} & 0.87 & 1.51 & 0.6 & 7.33 & 1.89 & 1 & 1 & 2.43 \\ \hline
        \textbf{rc-bd} & 1.12 & 1.92 & 0.39 & 7.96 & 2.28 & 1 & 1 & 3 \\ \hline
    \end{tabular}
    
    }
\end{table}

\begin{table}[!ht]
    \centering
    \caption{\textbf{Dataset}: Compas.  \textbf{Setting}: Ensemble - Filtering - Dominance Relation - Nadir Selection. \textbf{Removed element}: None }
    \makebox[0cm]{
    
    \begin{tabular}{|l|l|l|l|l|l|l|l|l|}
    \hline
        \textbf{Method} & \textbf{proximity} & \textbf{feasibility} & \textbf{discriminative\_power} & \textbf{sparsity} & \textbf{instability} & \textbf{coverage} & \textbf{actionable} & \textbf{rank} \\ \hline
        \textbf{dice} & 0.91 & 0.76 & 0.37 & 1.67 & 1.21 & 1 & 1 & 2.86 \\ \hline
        \textbf{fimap} & 0.49 & 0.1 & 0.68 & 3.12 & 0.18 & 0.58 & 0.58 & 5.57 \\ \hline
        \textbf{cadex} & 0.29 & 0.24 & 0.15 & 2.78 & 0.36 & 0.97 & 0.97 & 5.71 \\ \hline
        \textbf{wachter} & 0.28 & 0.19 & 0.22 & 2.44 & 0.25 & 0.77 & 0.77 & 6 \\ \hline
        \textbf{cem} & 0.33 & 0.32 & 0.29 & 1.57 & 0.38 & 1 & 1 & 3.14 \\ \hline
        \textbf{cfproto} & 0.16 & 0.14 & 0.24 & 1.92 & 0.26 & 0.21 & 0.21 & 6.71 \\ \hline
        \textbf{growing-spheres} & 0.3 & 0.19 & 0.18 & 3.15 & 0.33 & 0.8 & 0.8 & 5.86 \\ \hline
        \textbf{actionable-recourse} & 0.07 & 0.32 & 0.89 & 1 & 0.66 & 0 & 0 & 5.57 \\ \hline
        \textbf{face} & 0.38 & 0.03 & 0.71 & 2.75 & 0.13 & 0.27 & 0.27 & 5.71 \\ \hline
        \textbf{ip-manhattan} & 0.54 & 0.12 & 0.87 & 2.4 & 0.28 & 1 & 1 & 2 \\ \hline
        \textbf{ip-euclidean} & 0.54 & 0.13 & 0.86 & 2.43 & 0.28 & 1 & 1 & 2.29 \\ \hline
        \textbf{ip-chebyshev} & 0.55 & 0.15 & 0.86 & 2.48 & 0.28 & 1 & 1 & 2.29 \\ \hline
        \textbf{s-bd} & 0.54 & 0.12 & 0.87 & 2.4 & 0.28 & 1 & 1 & 2 \\ \hline
        \textbf{rc-bd} & 0.62 & 0.48 & 0.31 & 2.36 & 0.76 & 1 & 1 & 3 \\ \hline
    \end{tabular}
    
    }
\end{table}
