# Supplementary material for: A multi-criteria approach for selecting an explanation from the set of counterfactuals produced by an ensemble of explainers
Source: arXiv:2403.13940 source file (2024-08-02)
Supplement: Supplementary file 4 [file elements_study_on_filtered.tex]

\begin{table}[!ht]
    \centering
    \caption{\textbf{Dataset}: German. \textbf{Setting}: Ensemble - Dominance Relation - Ideal Point Selection. \textbf{Removed element}: Filtering}
    \makebox[0cm]{
    
    \begin{tabular}{|l|l|l|l|l|l|l|l|l|l|}
    \hline
        \textbf{Method} & \textbf{proximity} & \textbf{feasibility} & \textbf{discriminative\_power} & \textbf{sparsity} & \textbf{instability} & \textbf{coverage} & \textbf{validity} & \textbf{actionable} & \textbf{rank} \\ \hline
        \textbf{dice} & 1.93 & 4.02 & 0.43 & 2.18 & 4.34 & 1 & 1 & 1 & 4.12 \\ \hline
        \textbf{cadex} & 1.34 & 3.71 & 0.45 & 2.73 & 3.84 & 1 & 0.81 & 1 & 4 \\ \hline
        \textbf{fimap} & 6.58 & 2.96 & 0.76 & 9.78 & 3.65 & 1 & 0.57 & 1 & 2.88 \\ \hline
        \textbf{wachter} & 0.68 & 3.5 & 0.61 & 3.29 & 3.67 & 1 & 0.2 & 1 & 3.38 \\ \hline
        \textbf{cem} & 0.39 & 3.55 & 0.65 & 1.61 & 3.75 & 1 & 0.13 & 1 & 3.12 \\ \hline
        \textbf{cfproto} & 4.18 & 4.55 & 0.48 & 5.65 & 4.62 & 1 & 0.97 & 0.87 & 5.5 \\ \hline
        \textbf{growing-spheres} & 7.38 & 5.76 & 0.57 & 10.43 & 5.29 & 1 & 0.65 & 1 & 3.5 \\ \hline
        \textbf{actionable-recourse} & 0.67 & 3.38 & 0.46 & 0.94 & 3.4 & 0.36 & 0.87 & 0.36 & 7.62 \\ \hline
        \textbf{face} & 5.05 & 1.87 & 0.62 & 8.19 & 3.75 & 1 & 0.99 & 0.98 & 4.5 \\ \hline
        \textbf{s-op} & 3.19 & 2.12 & 0.9 & 5.77 & 3.41 & 1 & 0.64 & 0.98 & 3.75 \\ \hline
        \textbf{s-bd} & 2.2 & 2.63 & 0.92 & 4.51 & 3.58 & 1 & 0.48 & 0.98 & 3.5 \\ \hline
        \textbf{ip-manhattan} & 2.2 & 2.63 & 0.92 & 0.92 & 3.58 & 1 & 0.48 & 0.98 & 3.5 \\ \hline
        \textbf{ip-euclidean} & 1.65 & 2.83 & 0.87 & 3.57 & 3.66 & 1 & 0.53 & 0.99 & 3.62 \\ \hline
        \textbf{ip-chebyshev} & 1.76 & 2.86 & 0.82 & 3.48 & 3.65 & 1 & 0.57 & 0.99 & 3.75 \\ \hline
        \textbf{rc-op} & 2.86 & 2.64 & 0.68 & 4.95 & 3.43 & 1 & 0.7 & 1 & 3 \\ \hline
        \textbf{rc-bd} & 3.9 & 3.86 & 0.54 & 5.99 & 4.26 & 1 & 0.75 & 1 & 3.62 \\ \hline
    \end{tabular}
    
    }
\end{table}

\begin{table}[!ht]
    \centering
    \caption{\textbf{Dataset}: Adult. \textbf{Setting}: Ensemble - Dominance Relation - Ideal Point Selection. \textbf{Removed element}: Filtering}
    \makebox[0cm]{
    
    \begin{tabular}{|l|l|l|l|l|l|l|l|l|l|}
    \hline
        \textbf{Method} & \textbf{proximity} & \textbf{feasibility} & \textbf{discriminative\_power} & \textbf{sparsity} & \textbf{instability} & \textbf{coverage} & \textbf{validity} & \textbf{actionable} & \textbf{rank} \\ \hline
        \textbf{dice} & 1.14 & 0.88 & 0.35 & 1.74 & 1.23 & 1 & 1 & 1 & 3.88 \\ \hline
        \textbf{fimap} & 2.06 & 0.39 & 0.67 & 5.74 & 1.14 & 1 & 0.79 & 1 & 3.12 \\ \hline
        \textbf{cadex} & 0.21 & 0.3 & 0.19 & 2.38 & 0.64 & 0.99 & 0.98 & 0.99 & 6.12 \\ \hline
        \textbf{wachter} & 0.69 & 0.43 & 0.64 & 3.32 & 0.83 & 0.96 & 0.54 & 0.96 & 6 \\ \hline
        \textbf{cem} & 0.13 & 0.31 & 0.39 & 1.16 & 0.67 & 1 & 0.66 & 1 & 3.75 \\ \hline
        \textbf{cfproto} & 2.09 & 1.51 & 0.31 & 3.02 & 1.82 & 0.99 & 0.99 & 0.1 & 7.38 \\ \hline
        \textbf{growing-spheres} & 2.7 & 1.38 & 0.47 & 6.02 & 1.59 & 1 & 0.79 & 1 & 3.62 \\ \hline
        \textbf{face} & 1.16 & 0.09 & 0.69 & 3.8 & 0.57 & 1 & 0.96 & 0.82 & 4.5 \\ \hline
        \textbf{actionable-recourse} & 0.66 & 0.66 & 0.69 & 1.72 & 0.91 & 0.4 & 0.7 & 0.4 & 6.38 \\ \hline
        \textbf{s-op} & 0.66 & 0.1 & 0.94 & 2.82 & 0.54 & 1 & 0.53 & 0.9 & 4.12 \\ \hline
        \textbf{s-bd} & 0.45 & 0.16 & 0.99 & 2.61 & 0.61 & 1 & 0.27 & 0.94 & 3.25 \\ \hline
        \textbf{ip-manhattan} & 0.45 & 0.16 & 0.99 & 2.61 & 0.61 & 1 & 0.27 & 0.94 & 3.25 \\ \hline
        \textbf{ip-euclidean} & 0.36 & 0.21 & 0.97 & 2.5 & 0.62 & 1 & 0.24 & 0.97 & 3.12 \\ \hline
        \textbf{ip-chebyshev} & 0.36 & 0.22 & 0.96 & 2.53 & 0.62 & 1 & 0.24 & 0.97 & 3.25 \\ \hline
        \textbf{rc-op} & 0.71 & 0.2 & 0.67 & 2.67 & 0.6 & 1 & 0.73 & 0.93 & 4.38 \\ \hline
        \textbf{rc-bd} & 1.51 & 0.76 & 0.5 & 3.73 & 1.12 & 1 & 0.86 & 0.88 & 5 \\ \hline
    \end{tabular}
    
    }
\end{table}

\begin{table}[!ht]
    \centering
    \caption{\textbf{Dataset}: Fico. \textbf{Setting}: Ensemble - Dominance Relation - Ideal Point Selection. \textbf{Removed element}: Filtering}
    \makebox[0cm]{
    
   \begin{tabular}{|l|l|l|l|l|l|l|l|l|l|}
    \hline
        \textbf{Method} & \textbf{proximity} & \textbf{feasibility} & \textbf{discriminative\_power} & \textbf{sparsity} & \textbf{instability} & \textbf{coverage} & \textbf{validity} & \textbf{actionable} & \textbf{rank} \\ \hline
        \textbf{dice} & 1.14 & 2.18 & 0.36 & 1.99 & 2.54 & 1 & 1 & 1 & 4 \\ \hline
        \textbf{cadex} & 0.86 & 1.7 & 0.46 & 7.26 & 2.04 & 1 & 0.85 & 1 & 3.75 \\ \hline
        \textbf{fimap} & 1.39 & 1.74 & 0.6 & 15.62 & 1.85 & 1 & 0.85 & 0.62 & 4.38 \\ \hline
        \textbf{wachter} & 0.91 & 1.67 & 0.47 & 13.72 & 1.88 & 1 & 0.69 & 1 & 3.62 \\ \hline
        \textbf{cem} & 1.12 & 2.08 & 0.5 & 5.8 & 2.47 & 1 & 1 & 1 & 3.38 \\ \hline
        \textbf{cfproto} & 0.79 & 1.55 & 0.46 & 10.63 & 1.82 & 1 & 0.7 & 0.49 & 5.25 \\ \hline
        \textbf{growing-spheres} & 1.38 & 1.88 & 0.53 & 16.26 & 2.4 & 1 & 0.54 & 1 & 3.25 \\ \hline
        \textbf{face} & 2.34 & 0.83 & 0.69 & 17.98 & 1.82 & 1 & 0.99 & 0.02 & 4.62 \\ \hline
        \textbf{s-op} & 1.42 & 1.13 & 0.93 & 11.98 & 1.7 & 1 & 0.58 & 0.48 & 3.88 \\ \hline
        \textbf{s-bd} & 0.88 & 1.43 & 0.9 & 8 & 1.86 & 1 & 0.36 & 0.78 & 3.38 \\ \hline
        \textbf{ip-manhattan} & 0.88 & 1.43 & 0.9 & 8 & 1.86 & 1 & 0.36 & 0.78 & 3.38 \\ \hline
        \textbf{ip-euclidean} & 0.79 & 1.47 & 0.86 & 9.04 & 1.85 & 1 & 0.35 & 0.86 & 3.38 \\ \hline
        \textbf{ip-chebyshev} & 0.88 & 1.46 & 0.8 & 10.33 & 1.83 & 1 & 0.4 & 0.89 & 3.38 \\ \hline
        \textbf{rc-op} & 1.32 & 1.26 & 0.68 & 11.49 & 1.85 & 1 & 0.68 & 0.56 & 4.38 \\ \hline
        \textbf{rc-bd} & 1.32 & 1.77 & 0.49 & 11.14 & 2.22 & 1 & 0.78 & 0.84 & 4.38 \\ \hline
    \end{tabular}
    
    }
\end{table}

\begin{table}[!ht]
    \centering
    \caption{\textbf{Dataset}: Compas. \textbf{Setting}: Ensemble - Dominance Relation - Ideal Point Selection. \textbf{Removed element}: Filtering}
    \makebox[0cm]{
    
     \begin{tabular}{|l|l|l|l|l|l|l|l|l|l|}
    \hline
        \textbf{Method} & \textbf{proximity} & \textbf{feasibility} & \textbf{discriminative\_power} & \textbf{sparsity} & \textbf{instability} & \textbf{coverage} & \textbf{validity} & \textbf{actionable} & \textbf{rank} \\ \hline
        \textbf{dice} & 0.96 & 0.84 & 0.36 & 1.7 & 1.3 & 1 & 1 & 1 & 3.88 \\ \hline
        \textbf{fimap} & 0.5 & 0.11 & 0.7 & 3.48 & 0.18 & 1 & 0.92 & 0.59 & 4.38 \\ \hline
        \textbf{cadex} & 0.26 & 0.22 & 0.32 & 2.66 & 0.33 & 1 & 0.81 & 0.99 & 4.5 \\ \hline
        \textbf{wachter} & 0.24 & 0.17 & 0.46 & 2.26 & 0.22 & 1 & 0.62 & 1 & 3.62 \\ \hline
        \textbf{cem} & 0.33 & 0.32 & 0.29 & 1.57 & 0.38 & 1 & 1 & 1 & 4.12 \\ \hline
        \textbf{cfproto} & 0.75 & 0.19 & 0.51 & 2.92 & 0.35 & 1 & 0.6 & 0.35 & 5.12 \\ \hline
        \textbf{growing-spheres} & 0.26 & 0.18 & 0.67 & 2.96 & 0.3 & 1 & 0.42 & 1 & 3.25 \\ \hline
        \textbf{actionable-recourse} & 0.01 & 0.08 & 0.44 & 0.14 & 0.15 & 0.03 & 0.98 & 0.03 & 7.5 \\ \hline
        \textbf{face} & 0.54 & 0.05 & 0.69 & 3.54 & 0.17 & 1 & 1 & 0.04 & 4.88 \\ \hline
        \textbf{s-op} & 0.29 & 0.07 & 0.96 & 2.68 & 0.19 & 1 & 0.38 & 0.65 & 4 \\ \hline
        \textbf{s-bd} & 0.22 & 0.1 & 0.99 & 2.38 & 0.22 & 1 & 0.22 & 0.83 & 2.75 \\ \hline
        \textbf{ip-manhattan} & 0.22 & 0.1 & 0.99 & 2.38 & 0.22 & 1 & 0.22 & 0.83 & 2.75 \\ \hline
        \textbf{ip-euclidean} & 0.22 & 0.1 & 0.99 & 2.48 & 0.22 & 1 & 0.2 & 0.83 & 2.75 \\ \hline
        \textbf{ip-chebyshev} & 0.22 & 0.1 & 0.98 & 2.5 & 0.22 & 1 & 0.2 & 0.82 & 3.5 \\ \hline
        \textbf{rc-op} & 0.39 & 0.07 & 0.73 & 2.98 & 0.16 & 1 & 0.75 & 0.44 & 4.38 \\ \hline
        \textbf{rc-bd} & 0.5 & 0.3 & 0.54 & 2.63 & 0.5 & 1 & 0.77 & 0.79 & 4.38 \\ \hline
    \end{tabular}
    
    }
\end{table}
